# Supplementary material for: Discovery of Endianness and Instruction Size Characteristics in Binary Programs from Unknown Instruction Set Architectures
Source: arXiv:2410.21558 source file (2024-10-28)
Supplement: Supplementary file 1 [file labels.tex]

\subsection{Labels}\label{appendix:labels}
\begin{longtable}{|l|l|l|l|l|}
    \hline
        \textbf{IsaDetect} & \textbf{CpuRec} & \textbf{Wordsize} & \textbf{Endianness} & \textbf{Instruction Size} \\ \hline
~          & 6502.corpus        & 8        & LE & 8-32 \\ \hline  
~          & 68hc08.corpus      & 8        & BE & 8-16 \\ \hline  
~          & 68hc11.corpus      & 8        & BE & 8-40 \\ \hline  
~          & 8051.corpus        & 32       & LE & 8-128 \\ \hline 
arm64      & arm64.corpus       & 64       & LE & 32 \\ \hline    
~          & armeb.corpus       & 32       & BE & 32 \\ \hline    
armel      & armel.corpus       & 32       & LE & 32 \\ \hline    
armhf      & armhf.corpus       & 32       & LE & 32 \\ \hline    
~          & arcompact.corpus   & 32       & LE & 16-32 \\ \hline 
~          & avr.corpus         & 8        & LE & 16-32 \\ \hline 
alpha      & alpha.corpus       & 64       & LE & 32 \\ \hline    
~          & axiscris.corpus    & 32       & LE & 16 \\ \hline    
~          & blackfin.corpus    & 32       & LE & 16-32 \\ \hline 
~          & clipper.corpus     & 32       & LE & 2-8 \\ \hline   
~          & cuda.corpus        & 32       & LE & 32 \\ \hline    
~          & cell-spu.corpus    & 32       & BE & 32 \\ \hline    
~          & compactrisc.corpus & 16       & LE & 16 \\ \hline    
~          & cray.corpus        & 64       & NA & ~ \\ \hline     
~          & epiphany.corpus    & 32       & LE & 16-32 \\ \hline 
~          & fr-v.corpus        & 32       & NA & ~ \\ \hline     
~          & fr30.corpus        & 32       & BE & 16 \\ \hline    
~          & ft32.corpus        & 32       & NA & ~ \\ \hline     
~          & h8-300.corpus      & 8        & BE & 8-16 \\ \hline  
~          & h8s.corpus         & 16       & BE & ~ \\ \hline     
~          & hp-focus.corpus    & 32       & NA & ~ \\ \hline     
hppa       & hp-pa.corpus       & 64       & BE & 32 \\ \hline    
~          & ia-64.corpus       & 64       & LE & 128 \\ \hline   
~          & iq2000.corpus      & 32       & BE & ~ \\ \hline     
~          & m32c.corpus        & 32       & NA & ~ \\ \hline     
~          & m32r.corpus        & 32       & BI & 16-32 \\ \hline 
m68k       & m68k.corpus        & 32       & BE & ~ \\ \hline     
~          & m88k.corpus        & 32       & BI & 32 \\ \hline    
~          & mcore.corpus       & 32       & BE & 16 \\ \hline    
mips64el   & ~                  & 64       & LE & 32 \\ \hline    
~          & mips16.corpus      & 16       & BI & 16 \\ \hline    
mips       & mipseb.corpus      & 32       & BE & 32 \\ \hline    
mipsel     & mipsel.corpus      & 32       & LE & 32 \\ \hline    
~          & mmix.corpus        & 64       & BE & 32 \\ \hline    
~          & mn10300.corpus     & 32       & LE & ~ \\ \hline     
~          & msp430.corpus      & 16       & LE & ~ \\ \hline     
~          & mico32.corpus      & 32       & BE & 32 \\ \hline    
~          & microblaze.corpus  & 32/64    & BI & 32 \\ \hline    
~          & moxie.corpus       & 32       & BI & 32-48 \\ \hline 
~          & nds32.corpus       & 32/16    & BI & 16-32 \\ \hline 
~          & nios-ii.corpus     & 32       & LE & 32 \\ \hline    
~          & ocaml.corpus       & NA       & NA & ~ \\ \hline     
~          & pdp-11.corpus      & 16       & LE & 16 \\ \hline    
~          & pic10.corpus       & 8        & LE & ~ \\ \hline     
~          & pic16.corpus       & 8        & LE & ~ \\ \hline     
~          & pic18.corpus       & 8        & LE & ~ \\ \hline     
~          & pic24.corpus       & 16       & LE & 24 \\ \hline    
ppc64      & ppceb.corpus       & 64       & BE & ~ \\ \hline     
ppc64el    & ppcel.corpus       & 64       & LE & ~ \\ \hline     
riscv64    & risc-v.corpus      & 64       & LE & 32 \\ \hline    
~          & rl78.corpus        & 16       & LE & ~ \\ \hline     
~          & romp.corpus        & 32       & BE & 8-32 \\ \hline  
~          & rx.corpus          & 16/32/64 & LE & ~ \\ \hline     
s390x      & ~                  & 64       & BE & ~ \\ \hline     
s390       & s-390.corpus       & 32       & BE & ~ \\ \hline     
sparc      & ~                  & 32       & BE & 32 \\ \hline    
sparc64    & sparc.corpus       & 64       & BE & 32 \\ \hline    
~          & stm8.corpus        & 8        & ~  & ~ \\ \hline     
~          & stormy16.corpus    & 16       & LE & ~ \\ \hline     
sh4        & superh.corpus      & 32       & BI & ~ \\ \hline     
~          & tilepro.corpus     & 32       & ~  & ~ \\ \hline     
~          & tlcs-90.corpus     & 8        & ~  & ~ \\ \hline     
~          & tms320c2x.corpus   & 16/32    & ~  & ~ \\ \hline     
~          & tms320c6x.corpus   & 32       & BI & ~ \\ \hline     
~          & trimedia.corpus    & ~        & ~  & ~ \\ \hline     
~          & v850.corpus        & 32       & ~  & ~ \\ \hline     
~          & visium.corpus      & 32       & ~  & ~ \\ \hline     
~          & wasm.corpus        & 32       & LE & ~ \\ \hline     
~          & we32000.corpus     & 32       & ~  & ~ \\ \hline     
amd64      & x86-64.corpus      & 64       & LE & 8-120 \\ \hline 
i386       & x86.corpus         & 32       & LE & 8-120 \\ \hline 
~          & xtensa.corpus      & 32       & BI & 16-24 \\ \hline 
~          & z80.corpus         & 8        & LE & 8-32 \\ \hline  
~          & i860.corpus        & 32/64    & BI & ~ \\ \hline     
ia64       & ~                  & 64       & LE & 128 \\ \hline   
x32        & ~                  & 32       & LE & ~ \\ \hline     
powerpc    & ~                  & 32       & BE & 32 \\ \hline    
powerpcspe & ~                  & 32       & BE & 32 \\ \hline    
~          & 78k.corpus         & 8 or 16  & ~  & ~ \\ \hline    
\end{longtable}
