# Supplementary material for: Discovery of Endianness and Instruction Size Characteristics in Binary Programs from Unknown Instruction Set Architectures
Source: arXiv:2410.21558 source file (2024-10-28)
Supplement: Supplementary file 2 [file parameter_tuning.tex]

\subsection{Parameter tuning}\label{appendix:parameter_tuning}

\newcommand{\hyperparmcaptionnodot}[5]{Comparison of \MakeLowercase{{#1}} for the {#4} feature. Detection of {#2}. Trained and tested on {#3}, with {#5} files per ISA}

\newcommand{\hyperparmcaptionvar}[9]{\hyperparmcaptionnodot{#1}{#2}{#3}{#4}{#5}, with powers of {#6} of the \texttt{\MakeLowercase{{#7}}} parameter from {#8} to {#9}.}

\newcommand{\hyperparmcaptionentirenodot}[4]{Comparison of \MakeLowercase{{#1}} for the {#4} feature. Detection of {#2}. Trained and tested on the entire {#3} dataset}

\newcommand{\hyperparmcaptionentirevarnodot}[8]{\hyperparmcaptionentirenodot{#1}{#2}{#3}{#4} with powers of {#5} of the \texttt{\MakeLowercase{{#6}}} parameter from {#7} to {#8}}
\newcommand{\hyperparmcaptionentirevar}[8]{\hyperparmcaptionentirevarnodot{#1}{#2}{#3}{#4}{#5}{#6}{#7}{#8}.}

\subsubsection{Feature parameter tuning}\label{appendix:feature_parameter_tuning}
\paragraph{Fixed/Variable instruction size - AutoCorrelation}
\begin{figure}[H]
    \centering
    \includegraphics[width=0.8\linewidth]{Images/40_Results/autocorr_tuning/isvar_AutoCorrelation.png}
    \caption{\hyperparmcaptionentirevar{\texttt{Lag}}{fixed/variable instruction size}{CpuRec}{AutoCorrelation}{two}{\texttt{Lag}}{16}{1024}}
    \label{fig:featureparam Fixed/Variable instruction size - AutoCorrelation}
\end{figure}

\paragraph{Fixed/Variable instruction size - Fourier}
\begin{figure}[H]
    \centering
    \includegraphics[width=0.8\linewidth]{Images/40_Results/fourier_tuning/isvar_None_Fourier.png}
    \caption{\hyperparmcaptionentirevar{\texttt{data\_half\_len}}{fixed/variable instruction size}{CpuRec}{Fourier}{two}{\texttt{data\_half\_len}}{16}{1024} Note that \texttt{data\_half\_len} for the SVC classifier are no lower than 32, as lower frequencies drastically increase training time.}
    \label{fig:featureparam Fixed/Variable instruction size - Fourier}
\end{figure}

\paragraph{Fixed instruction size - AutoCorrelation}
\begin{figure}[H]
    \centering
    \includegraphics[width=0.8\linewidth]{Images/40_Results/autocorr_tuning/instsize_AutoCorrelation.png}
    \caption{\hyperparmcaptionentirevar{\texttt{Lag}}{fixed instruction size}{CpuRec}{AutoCorrelation}{two}{\texttt{Lag}}{16}{512}}
    \label{fig:featureparam Fixed instruction size - AutoCorrelation}
\end{figure}

\paragraph{Fixed instruction size - Fourier}
\begin{figure}[H]
    \centering
    \includegraphics[width=0.8\linewidth]{Images/40_Results/fourier_tuning/instsize_None_Fourier.png}
    \caption{\hyperparmcaptionentirevar{\texttt{data\_half\_len}}{fixed instruction size}{CpuRec}{Fourier}{two}{\texttt{data\_half\_len}}{16}{1024}}
    \label{fig:featureparam Fixed instruction size - Fourier}
\end{figure}

\subsubsection{Classifier hyperparameter tuning}\label{appendix:hyperparameter_tuning}
\paragraph{Endianness - 100 files per architecture}
\begin{figure}[H]
    \centering
    \includegraphics[width=0.8\linewidth]{Images/40_Results/hyperparameter_tuning/endianness_full_100_EndiannessSignatures.png}
    \caption{\hyperparmcaptionvar{Hyperparameters}{endianness detection}{IsaDetectFull}{endianness signatures}{100}{ten}{c}{$10^{1}$}{$10^{11}$}}
    \label{fig:hyperparam Endianness, endianness signatures, full - 100}
\end{figure}

\paragraph{Endianness}
\begin{figure}[H]
    \centering
    \includegraphics[width=0.8\linewidth]{Images/40_Results/hyperparameter_tuning/endianness_full_30_EndiannessSignatures.png}
    \caption{\hyperparmcaptionvar{Hyperparameters}{endianness detection}{IsaDetectFull}{endianness signatures}{30}{ten}{c}{$10^{1}$}{$10^{11}$}}
    \label{fig:hyperparam Endianness, endianness signatures, full}
\end{figure}

\begin{figure}[H]
    \centering
    \includegraphics[width=0.8\linewidth]{Images/40_Results/hyperparameter_tuning/endianness_full_30_Bigrams.png}
    \caption{\hyperparmcaptionvar{Hyperparameters}{endianness detection}{IsaDetectFull}{bigrams}{30}{ten}{c}{$10^{1}$}{$10^{10}$}}
    \label{fig:hyperparam Endianness, bigrams, full}
\end{figure}

\begin{figure}[H]
    \centering
    \includegraphics[width=0.8\linewidth]{Images/40_Results/hyperparameter_tuning/endianness_code_30_EndiannessSignatures.png}
    \caption{\hyperparmcaptionvar{Hyperparameters}{endianness detection}{IsaDetectCode}{endianness signatures}{30}{ten}{c}{$10^{1}$}{$10^{11}$}}
    \label{fig:hyperparam Endianness, endianness signatures, code}
\end{figure}

\begin{figure}[H]
    \centering
    \includegraphics[width=0.8\linewidth]{Images/40_Results/hyperparameter_tuning/endianness_code_30_Bigrams.png}
    \caption{\hyperparmcaptionvar{Hyperparameters}{endianness detection}{IsaDetectCode}{bigrams}{30}{ten}{c}{$10^{1}$}{$10^{10}$}}
    \label{fig:hyperparam Endianness, bigrams, code}
\end{figure}

\paragraph{Fixed/variable instruction size}
\begin{figure}[H]
    \centering
    \includegraphics[width=0.8\linewidth]{Images/40_Results/hyperparameter_tuning/isvar_None_ByteDifferencePrimes.png}
    \caption{\hyperparmcaptionentirevar{Hyperparameters}{fixed/variable instruction size}{CpuRec}{ByteDifferencePrimes}{ten}{\texttt{c}}{$10^{-4}$}{$10^6$}}
    \label{fig:hyperparam isvar, ByteDifferencePrimes}
\end{figure}

\begin{figure}[H]
    \centering
    \includegraphics[width=0.8\linewidth]{Images/40_Results/hyperparameter_tuning/isvar_None_AutoCorrelation_1-32.png}
    \caption{\hyperparmcaptionentirevar{Hyperparameters}{fixed/variable instruction size}{CpuRec}{AutoCorrelation}{ten}{\texttt{c}}{$10^{-1}$}{$10^6$}}
    \label{fig:hyperparam isvar, AutoCorrelation}
\end{figure}

\begin{figure}[H]
    \centering
    \includegraphics[width=0.8\linewidth]{Images/40_Results/hyperparameter_tuning/isvar_None_Fourier.png}
    \caption{\hyperparmcaptionentirevar{Hyperparameters}{fixed/variable instruction size}{CpuRec}{Fourier}{ten}{\texttt{c}}{$10^{-7}$}{$10^9$}}
    \label{fig:hyperparam isvar, Fourier}
\end{figure}

\paragraph{Fixed instruction size}

\begin{figure}[H]
    \centering
    \includegraphics[width=0.8\linewidth]{Images/40_Results/hyperparameter_tuning/instsize_None_AutoCorrelation.png}
    \caption{\hyperparmcaptionentirevar{Hyperparameters}{fixed instruction size}{CpuRec}{AutoCorrelation}{ten}{\texttt{c}}{$10^{-7}$}{$10^7$}}
    \label{fig:hyperparam instsize, AutoCorrelation}
\end{figure}

\begin{figure}[H]
    \centering
    \includegraphics[width=0.8\linewidth]{Images/40_Results/hyperparameter_tuning/instsize_None_Fourier.png}
    \caption{\hyperparmcaptionentirevar{Hyperparameters}{fixed instruction size}{CpuRec}{Fourier}{ten}{\texttt{c}}{$10^{-7}$}{$10^9$}}
    \label{fig:hyperparam instsize, Fourier}
\end{figure}

\begin{figure}[H]
    \centering
    \includegraphics[width=0.8\linewidth]{Images/40_Results/hyperparameter_tuning/instsize_None_AutoCorrelationPeak3_1-32.png}
    \caption{\hyperparmcaptionentirevar{Hyperparameters}{fixed instruction size}{CpuRec}{Fourier}{ten}{\texttt{c}}{$10^{-7}$}{$10^7$}}
    \label{fig:hyperparam instsize, AutoCorrelationPeak3}
\end{figure}
