# Supplementary material for: Discovery of Endianness and Instruction Size Characteristics in Binary Programs from Unknown Instruction Set Architectures
Source: arXiv:2410.21558 source file (2024-10-28)
Supplement: Supplementary file 3 [file baselines.tex]

\subsection{Baselines}\label{appendix:baselines}
\begin{table}[H]
    \centering
    \begin{tabular}{|l||c||c|c|}
        \hline
        \multirow{2}{*}{\textbf{ISA feature}} & \textbf{CpuRec} & \textbf{IsaDetect} & \textbf{IsaDetect} \\
        & \textbf{baseline} & \textbf{baseline - all} & \textbf{baseline - x specified} \\
        \hline
         \textbf{Endianness} & $33/51 = \textbf{0.647}$ & $50287/90465 = \textbf{0.556}$ & $12x/22x = \textbf{0.545}$ \\
        \hline
         \textbf{Fixed/variable} & \multirow{2}{*}{$25/43 = \textbf{0.581}$} & \multirow{2}{*}{$57356/66831 = \textbf{0.858}$} & \multirow{2}{*}{$14x/16x = \textbf{0.875}$} \\ \textbf{instruction size} & & & \\
         \hline
         \textbf{Fixed instruction size} & $17/25 = \textbf{0.680}$ & $52372/57356 = \textbf{0.913}$ & $13x/14x = \textbf{0.929}$ \\
        \hline
    \end{tabular}
\end{table}
