# Supplementary material for: Discovery of Endianness and Instruction Size Characteristics in Binary Programs from Unknown Instruction Set Architectures
Source: arXiv:2410.21558 source file (2024-10-28)
Supplement: Supplementary file 4 [file isa_feature_counts.tex]

\subsection{ISA feature counts}\label{appendix:isa_feature_counts}
\begin{table}[H]
    \centering
    \begin{tabular}{|l||c|c||c|c|}
        \hline
        \multirow{2}{*}{\textbf{ISA feature class}} & \textbf{CpuRec} & \textbf{CpuRec} & \textbf{IsaDetect} & \textbf{IsaDetect} \\
        & \textbf{class count} & \textbf{file count} & \textbf{class count} & \textbf{file count} \\
        \hline
         \textbf{Little endian} & 33 & 33 & 12 & 50287 \\
        \hline
         \textbf{Big endian} & 18 & 18 & 10 & 40178 \\
        \hline
         \textbf{Endianness total} & 51 & 51 & 22 & 90465 \\
        \hline
         \textbf{Instruction size 16} & 6 & 6 & 0 & 0 \\
         \hline
         \textbf{Instruction size 24} & 1 & 1 & 0 & 0 \\
         \hline
         \textbf{Instruction size 32} & 17 & 17 & 13 & 52372 \\
         \hline
         \textbf{Instruction size 128} & 1 & 1 & 1 & 4984 \\
        \hline
         \textbf{Fixed instruction size} & 25 & 25 & 14 & 57356 \\
        \hline
         \textbf{Variable instruction size} & 18 & 18 & 2 & 9475 \\
         \hline
         \textbf{Fixed/variable} & \multirow{2}{*}{43} & \multirow{2}{*}{43} & \multirow{2}{*}{16} & \multirow{2}{*}{66831} \\ \textbf{instruction size total} & & & & \\
        \hline
    \end{tabular}
\end{table}
