# Supplementary material for: Discovery of Endianness and Instruction Size Characteristics in Binary Programs from Unknown Instruction Set Architectures
Source: arXiv:2410.21558 source file (2024-10-28)
Supplement: Supplementary file 5 [file isadetect_filecounts.tex]

\subsection{IsaDetect file counts}\label{appendix:isadetect_filecounts}
\begin{table}[H]
    \centering
    \begin{tabular}{|c|c|}
\hline
\textbf{ISA}  & \textbf{File count}\\\hline
alpha         & 3971\\\hline
amd64         & 4366\\\hline
arm64         & 3636\\\hline
armel         & 4000\\\hline
armhf         & 3995\\\hline
hppa          & 4830\\\hline
i386          & 5109\\\hline
ia64          & 4984\\\hline
m68k          & 4400\\\hline
mips          & 3565\\\hline
mips64el      & 4312\\\hline
mipsel        & 3775\\\hline
powerpc       & 3631\\\hline
powerpcspe    & 3961\\\hline
ppc64         & 2833\\\hline
ppc64el       & 3523\\\hline
riscv64       & 4440\\\hline
s390          & 5164\\\hline
s390x         & 3538\\\hline
sh4           & 5930\\\hline
sparc         & 4980\\\hline
sparc64       & 3276\\\hline
x32           & 4176\\\hline
\hline
\textit{Total} & 96395\\\hline 
    \end{tabular}
    % \caption{Table of number of files for each ISA in the ISADetect datasets.}
\end{table}
